# Supplementary material for: FuSSI-Net: Fusion of Spatio-temporal Skeletons for Intention Prediction Network
Source: arXiv:2005.07796 source file (2020-05-15)
Supplement: Supplementary file 1 [file Supplementary_Materials.pdf]

## Supplementary Material

### A. Fusion Model Experiments on JAAD data

**Table 1: Densenet Experiments Using Adam Optimizer**

| Train Set | Test Set | 1e-4 Learning Rate Epoch Number | Metric | Original | Late Fusion | Early Fusion | Combination |
|---|---|---|---|---|---|---|---|
| JAAD Videos 1 to 230 | JAAD Videos 231 to 271 | 30 | Acc | 0.742 | 0.757 | 0.785 | 0.785 |
| | | | Loss | 0.674 | 0.740 | 0.668 | 0.719 |
| | | | AP | 0.810 | 0.806 | 0.872 | 0.741 |

The first step was to balance the unbalanced JAAD dataset by artificially creating more samples of the not-crossing sequences extracted from JAAD dataset. For each crossing pedestrian their last 16 frames were used as a test sequence whereas for a not-crossing pedestrian (pedestrians that were standing or walking in the direction parallel to the ego vehicle's motion), their entire sequence was sampled to get as many 16 frames as possible to balance the positive samples in the training dataset. We also opted for the more stable but slower training stochastic gradient descent optimizer. After more than 1000 epochs, the early fusion approach achieved an AP score of 0.891, an increase from the previously reported AP score of 0.845.

**Table 2: Densenet Experiments Using SGD Optimizer**

| Train Set | Test Set | Model | 1e-2 Learning Rate Epoch Number | 1e-3 Learning Rate Epoch Number | 1e-4 Learning Rate Epoch Number | Metric | Result |
|---|---|---|---|---|---|---|---|
| JAAD Artificially Balanced Set | JAAD Videos 299 to 346 | Original | 0 | 500 | 0 | Acc | 0.675 |
| | | | | | | Loss | 0.96 |
| | | | | | | AP | 0.828 |
| | | Early Fusion | 20 | | 500 | Acc | 0.756 |
| | | | | | | Loss | 0.93 |
| | | | | | | AP | 0.89 |

B. **Keypoint annotations of JAAD:** For the first 50 videos in JAAD, we annotated frame 0, 59, 119 etc. depending on the length of the video. We deleted the frame if it didn't contain any pedestrian. In total, we annotated 212 frames with up to 17 keypoints per pedestrian.

C. **Performance of Skeletal Fitting Model**

The videos selected for evaluation of the training with Coco-GAN frames were chosen to reflect an equal split between bright and dark conditions. This was done to measure the combined performance for both bright and dark conditions. For evaluation of the model trained on whole keypoint annotated JAAD images and cropped keypoint annotated JAAD images, videos were chosen at random in order to represent the
dataset in general, excluding the 50 first videos of JAAD. This was done since the model had been trained on frames from these videos.

| JAAD-videos for evaluation of Coco-GAN | JAAD-videos for evaluation of whole JAAD images and cropped JAAD images |
|---|---|
| video_0001 | video_0053 |
| video_0002 | video_0061 |
| video_0003 | video_0139 |
| video_0023* | video_0154 |
| video_0024* | video_0201 |
| video_0026* | video_0224 |
| Total frames (* represent night time videos): 1920 (960 dark+1020 bright) | Total frames: 1350 |

Table X: JAAD-videos chosen to evaluate skeleton fitting models

The 70 test sequences used to test the skeleton model correspond to the pedestrians in JAAD videos 231 to 271.

Results from running skeleton fitting as an independent object-detector. IOU threshold used during metric calculation: 0.3

| **JAAD-videos used for this benchmark:** | video_0053, video_0061, video_0139, video_0154, video_0201, video_0224 | | |
|---|---|---|---|
| | **Original implementation** | **Model retrained on whole JAAD images** | **Model retrained on cropped JAAD images** |

| | | | |
|---|---|---|---|
| Precision | 0.57 | 0.36 | 0.23 |
| Recall | 0.14 | 0.17 | 0.08 |
| AP | 11.37% | 7.79% | 6.16% |

**JAAD-videos used for this benchmark:** video_0001, video_0002, video_0003, video_0023*, video_0024*, video_0026 * *Dark condition videos

| Total evaluation | | |
|---|---|---|
| | **Original implementation** | **Model retrained on Coco-Gan images** |
| Precision | 0.57 | 0.13 |
| Recall | 0.21 | 0.06 |
| AP | 19.69% | 2.27% |
| **Dark conditions** | | |
| | **Original implementation** | **Model retrained on Coco-Gan images** |
| Precision | 0.17 | 0.14 |
| Recall | 0.03 | 0.07 |
| AP | 1.58% | 4.62% |
| **Bright conditions** | | |
| | **Original implementation** | **Model retrained on Coco-Gan images** |
| Precision | 0.69 | 0.11 |
| Recall | 0.46 | 0.04 |
| AP | 43.37% | 1.26% |

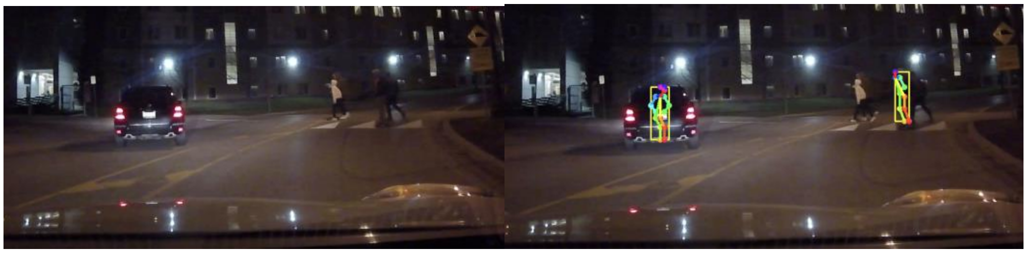

Figure 1. Left: Before retraining skeleton on COCO GAN. Right: After retraining on COCO-GAN

As shown in the above figure, the skeleton fitting model retrained on COCO-GAN is able to fit a skeleton onto a pedestrian, which the original model could not. Beware that the retrained model also detects a false positive in the trunk of the car, which the original model does not.

## D. YOLOv3 trained on CycleGAN Augmented JAAD dataset

An experiment was conducted to assess improvement in the performance of YOLOv3 object detector in low visibility and night time like conditions. The training and validation dataset was created from the same train and val split wherein the 20k images were augmented for training and 9k images were augmented for validation. Since, the total train and validation dataset would include the original images, the train dataset consists of 40,000 images and validation dataset consists of 18,000 images. The following figure displays the augmented and unaugmeted JAAD training instance. To test the performance of the YOLOv3 trained on such augmented dataset, 6 videos from JAAD are chosen such that 3 are daytime and 3 are night time videos.

**JAAD-videos used for this benchmark:** video_0001, video_0002, video_0003, video_0023*, video_0024*, video_0026 * (*Dark condition videos)

| **Total evaluation for all conditions** | | |
|---|---|---|
| | **Original implementation** | **Model retrained on JAAD-CyGAN images** |
| Precision | 0.97 | 0.92 |
| Recall | 0.48 | 0.45 |
| AP | 48.46% | 42.34% |
| **Dark conditions** | | |
| | **Original implementation** | **Model retrained on JAAD-CyGAN images** |
| Precision | 0.95 | 0.87 |
| Recall | 0.16 | 0.29 |
| AP | 16.01% | 28.49% |
| **Bright conditions** | | |
| | **Original implementation** | **Model retrained on JAAD-CyGAN images** |
| Precision | 0.98 | 0.95 |
| Recall | 0.90 | 0.65 |
| AP | 91.78% | 61.21% |

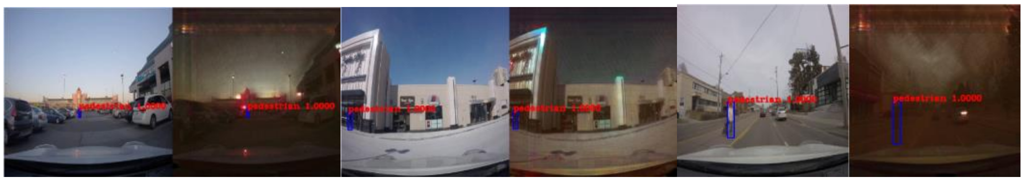

Figure 2. Original and augmented training instance with annotation.

## E. Evaluation and results of the classifiers:

To measure the performance of the classifiers a few different metrics were calculated: accuracy, precision and recall. ((The accuracy was calculated according to Equation 6, precision was calculated according to Equation 7 and recall according to Equation 8. In these cases, True Positives mean the number of correctly classified Crossing predictions, False Positives mean the number of incorrectly classified Crossing predictions, True Negatives mean the number of correctly classified Not Crossing predictions and False Negative mean the number of incorrectly classified Not Crossing predictions. Furthermore, the Total number of classifications is the sum of the True Positives, True Negatives, False Positives and False Negatives.))
The different metrics were calculated as an average over 12 separate training and test runs on the same train and test split of the data. The padding for the RNN was excluded from all metric calculations.
The metrics used in [4] were based on predictions only for pedestrians whose BB was at least 60 pixels wide. Also, as done in [4], labels {clear-path, slow- down, speed-up} for pedestrians with lateral motion direction are classified as C. Additionally, they balanced the set of predictions to get a fully accurate representation of the two predicted classes, since the Cross-classification appeared to be more
frequent in the prediction set. Therefore, the same methods to balance the data for metric calculations and excluding data from smaller BB:s were used in this report.

**Random Forest:**
The performance of the RF classifier was tested on the original skeleton model and the retrained one. The metrics accuracy, recall and precision were calculated, which can be found in table 7.

| Input data | Average Accuracy | Average Recall | Average Precision |
|---|---|---|---|
| Before retraining skeleton | 72.95% | 79.23% | 70.39% |
| After retraining skeleton | 74.09% | 84.32% | 70.00% |
| Results presented in X | 88% | - | - |

**RNN:**
Different model structures tested for RNN:

| Model number | | | |
|---|---|---|---|
| 1 | 2 | 3 | 4 |
| Bidirectional LSTM,<br>16 neurons,<br>BatchNormalization<br>0.1 dropout | LSTM,<br>16 neurons,<br>BatchNormalization<br>0.1 dropout | Bidirectional LSTM,<br>16 neurons,<br>BatchNormalization<br>0.1 dropout | Bidirectional LSTM,<br>16 neurons,<br>BatchNormalization<br>0.1 dropout |
| LSTM, 16 neurons,<br>BatchNormalization | LSTM, 16 neurons,<br>BatchNormalization | | LSTM, 16 neurons,<br>BatchNormalization |

| | | | |
|---|---|---|---|
| LSTM, 16 neurons, BatchNormalization | LSTM, 16 neurons, BatchNormalization | | LSTM, 16 neurons, BatchNormalization |
| | | | LSTM, 16 neurons, BatchNormalization |
| TimeDistributed Dense layer, 1 neuron, 0.2 dropout | Dense layer, 1 neuron, 0.2 dropout | TimeDistributed Dense layer, 1 neuron, 0.2 dropout | TimeDistributed Dense layer, 1 neuron, 0.2 dropout |

Different structures for the RNN were tested as can be seen in table 2. These models were further used in experiments of other parameters that affect the performance of the RNN. Table 8 shows the seven experiments conducted on the RNN classifier and their respective results. For more details on the models referred to in column 1, see table 2. In addition to benchmarking the different models, there were also experiments done to compare the results of using input data from the original skeleton model and the retrained one, as well as to compare different loss functions for the output layer and lastly different number of added crossing annotations before the actual crossing starts, to potentially get an earlier prediction.

| Model nr | Loss function | PT | Input data | Av. Accuracy | Av. Recall | Av. Precision |
|---|---|---|---|---|---|---|
| 1 | mae | 14 | Before retraining skeleton | 72.92% | 72.12% | 74.74% |
| 1 | mae | 14 | After retraining skeleton | 76.50% | 78.74% | 72.67% |
| 1 | mae | 1 | After retraining skeleton | 75.99% | 77.84% | 72.73% |
| 1 | binary cross entropy | 14 | After retraining skeleton | 72.19% | 71.79% | 73.15% |
| 2 | mae | 14 | After retraining skeleton | 73.87% | 75.31% | 71.08% |
| 3 | mae | 14 | After retraining skeleton | 76.31% | 78.34% | 72.74% |
| 4 | mae | 14 | After retraining skeleton | 75.92% | 77.84% | 72.53% |

Table x: The results for different RNN models. The model number refers to the structures in table xx, PT (prediction time) is the number of frames before the actual crossing that is labeled as crossing and the average for the accuracy, recall and precision is calculated over 12 separate training and test runs of the model on the same train-test-split of the data.

### F. Runtime Performances of Models

The FPS includes all the processing work right from detection to the display of the results on each frame, including the storage and retrieval of the sliding . The computation platform consists of Intel(R) Xeon(R) CPU @ 2.20GHz, Tesla P100-PCIE-8GB, 25 GB RAM and Google Colaboratory IDE. The end to end models ran on the same platform simultaneously.

| Model | FPS |
|---|---|
| A | 8 |
| B | 0.6 |
| C | 6 |
| D | 0.6 |

## G. End to End model architecture diagrams

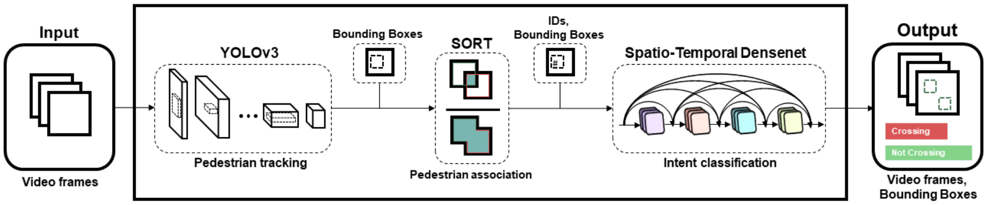


Figure 3. Model A

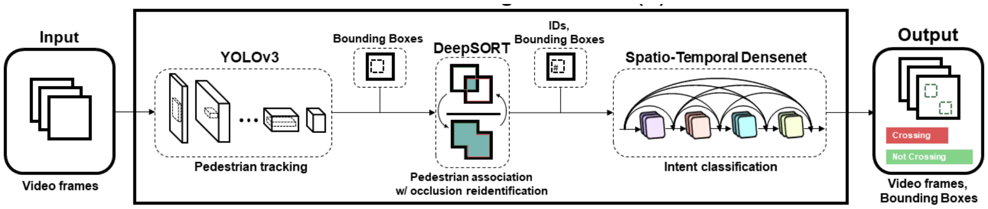


Figure 4. Model B

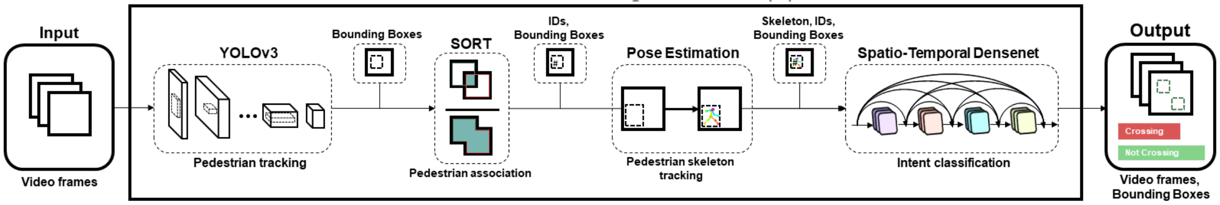


Figure 5. Model C

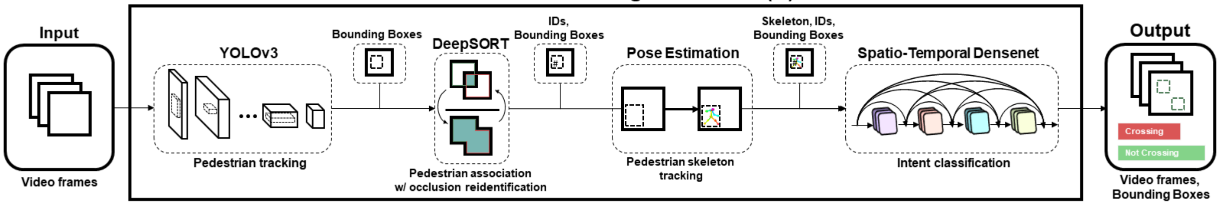

Figure 6. Model D

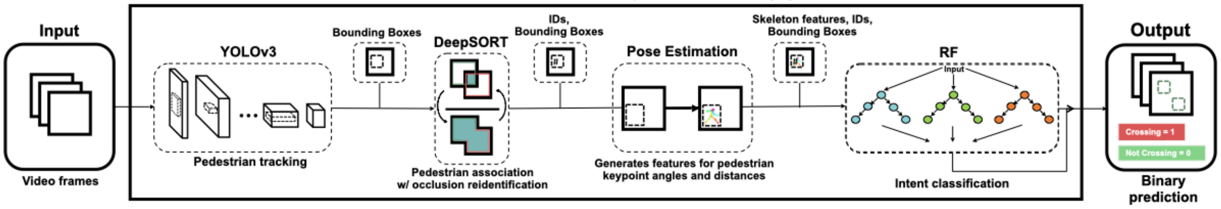


Figure 7. Model E

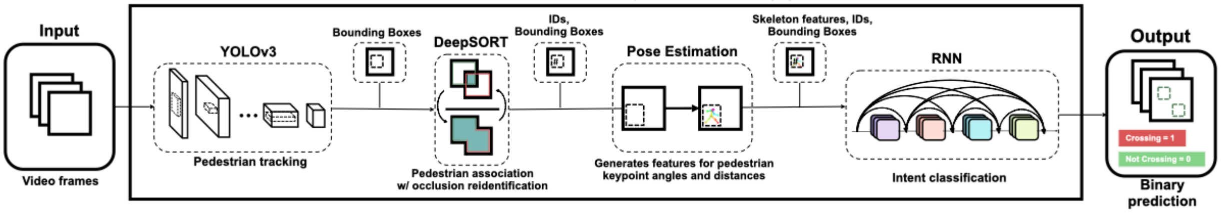


Figure 8. Model F
